# Supplementary material for: Bayesian Image Reconstruction and Uncertainty Quantification for Three-Photon Positronium Ratio Imaging: Toward Radiotheranostic Applications
Source: arXiv:2611.28333 source file (2026-11-25)
Supplement: Supplementary file 1 [file labels_supplement_SI.tex]

% generated by make_xref_labels.py from supplement_SI.aux: numbers of the supplement, used for \ref{S-...}
\makeatletter
\newlabel{S-app:gibbs}{{S14}{32}{}{}{}}
\newlabel{S-app:mlem}{{S15}{36}{}{}{}}
\newlabel{S-app:sqrt2}{{S16}{36}{}{}{}}
\newlabel{S-eq:cond}{{S12}{32}{}{}{}}
\newlabel{S-eq:s-cos}{{S2}{3}{}{}{}}
\newlabel{S-eq:s-cov}{{S7}{4}{}{}{}}
\newlabel{S-eq:s-dVdE}{{S4}{4}{}{}{}}
\newlabel{S-eq:s-dVdP}{{S6}{4}{}{}{}}
\newlabel{S-eq:s-dthdE}{{S5}{4}{}{}{}}
\newlabel{S-eq:s-f3}{{S17}{38}{}{}{}}
\newlabel{S-eq:s-g}{{S18}{38}{}{}{}}
\newlabel{S-eq:s-is}{{S9}{6}{}{}{}}
\newlabel{S-eq:s-op}{{S1}{2}{}{}{}}
\newlabel{S-eq:s-proj}{{S8}{5}{}{}{}}
\newlabel{S-eq:s-tienstra}{{S3}{4}{}{}{}}
\newlabel{S-eq:sqrt2}{{S16}{36}{}{}{}}
\newlabel{S-fig:attr}{{S1}{9}{}{}{}}
\newlabel{S-fig:eta}{{S5}{14}{}{}{}}
\newlabel{S-fig:images}{{S4}{12}{}{}{}}
\newlabel{S-fig:mcb}{{S2}{10}{}{}{}}
\newlabel{S-fig:rods}{{S6}{17}{}{}{}}
\newlabel{S-fig:s-poolrep}{{S7}{26}{}{}{}}
\newlabel{S-fig:s-priors}{{S8}{43}{}{}{}}
\newlabel{S-fig:sqrt2}{{S3}{11}{}{}{}}
\newlabel{S-prop:null}{{S1}{4}{}{}{}}
\newlabel{S-prop:s-bayes}{{S3}{29}{}{}{}}
\newlabel{S-prop:s-cz}{{S5}{30}{}{}{}}
\newlabel{S-prop:s-pg}{{S4}{30}{}{}{}}
\newlabel{S-prop:sum}{{S2}{5}{}{}{}}
\newlabel{S-sec:s-bayes}{{S5}{5}{}{}{}}
\newlabel{S-sec:s-cov}{{S6}{6}{}{}{}}
\newlabel{S-sec:s-extra}{{S7}{7}{}{}{}}
\newlabel{S-sec:s-fast}{{S10}{19}{}{}{}}
\newlabel{S-sec:s-g4like}{{S12}{23}{}{}{}}
\newlabel{S-sec:s-io}{{S8}{18}{}{}{}}
\newlabel{S-sec:s-jac}{{S3}{4}{}{}{}}
\newlabel{S-sec:s-mc}{{S1}{1}{}{}{}}
\newlabel{S-sec:s-priors}{{S17}{37}{}{}{}}
\newlabel{S-sec:s-real}{{S9}{18}{}{}{}}
\newlabel{S-sec:s-risk}{{S13}{29}{}{}{}}
\newlabel{S-sec:s-rods}{{S11}{20}{}{}{}}
\newlabel{S-sec:s-sum}{{S4}{5}{}{}{}}
\newlabel{S-sec:s-thera}{{S18}{44}{}{}{}}
\newlabel{S-sec:s-tienstra}{{S2}{3}{}{}{}}
\newlabel{S-tab:energy}{{S4}{10}{}{}{}}
\newlabel{S-tab:g4}{{S12}{22}{}{}{}}
\newlabel{S-tab:jmb}{{S3}{9}{}{}{}}
\newlabel{S-tab:p3d}{{S6}{15}{}{}{}}
\newlabel{S-tab:s-2g}{{S9}{20}{}{}{}}
\newlabel{S-tab:s-actions}{{S22}{40}{}{}{}}
\newlabel{S-tab:s-bench}{{S8}{20}{}{}{}}
\newlabel{S-tab:s-equiv}{{S20}{36}{}{}{}}
\newlabel{S-tab:s-eta}{{S5}{13}{}{}{}}
\newlabel{S-tab:s-event}{{S2}{7}{}{}{}}
\newlabel{S-tab:s-g4full}{{S15}{27}{}{}{}}
\newlabel{S-tab:s-loss}{{S16}{30}{}{}{}}
\newlabel{S-tab:s-matched-g4}{{S17}{33}{}{}{}}
\newlabel{S-tab:s-matched-real}{{S18}{34}{}{}{}}
\newlabel{S-tab:s-matched-real-sd}{{S19}{35}{}{}{}}
\newlabel{S-tab:s-mod}{{S11}{21}{}{}{}}
\newlabel{S-tab:s-pools}{{S14}{25}{}{}{}}
\newlabel{S-tab:s-priors-g4}{{S23}{41}{}{}{}}
\newlabel{S-tab:s-priors-phys-porous}{{S25}{42}{}{}{}}
\newlabel{S-tab:s-priors-porous}{{S21}{40}{}{}{}}
\newlabel{S-tab:s-priors-real}{{S24}{42}{}{}{}}
\newlabel{S-tab:s-realall}{{S13}{23}{}{}{}}
\newlabel{S-tab:s-rods}{{S7}{16}{}{}{}}
\newlabel{S-tab:s-scale}{{S10}{21}{}{}{}}
\newlabel{S-tab:s-thera}{{S27}{44}{}{}{}}
\newlabel{S-tab:s-valid}{{S1}{3}{}{}{}}
\newlabel{S-tab:s-voxel-g4}{{S26}{42}{}{}{}}
\makeatother
